# Supplementary material for: Elastic3D: Controllable Stereo Video Conversion with Guided Latent Decoding
Source: arXiv:2512.14236 source file (2026-07-09)
Supplement: Supplementary file 1 [file main_supplementary.tex]

\documentclass[10pt,twocolumn,letterpaper]{article}

\usepackage[review]{cvpr}      %

\input{preamble}

\usepackage{booktabs} %
\usepackage{graphicx} %
\usepackage{amsmath}  %
\usepackage{multirow}
\usepackage{pifont}
\usepackage[table]{xcolor}
\usepackage{arydshln}      %

\usepackage{multirow}
\usepackage{xfp}
\usepackage{overpic}

\usepackage{tikz}
\usetikzlibrary{spy, calc} %

\definecolor{cvprblue}{rgb}{0.21,0.49,0.74}
\usepackage[pagebackref,breaklinks,colorlinks,allcolors=cvprblue]{hyperref}

\title{Guided Latent Decoding for Controllable Stereo Video Conversion}

\author{First Author\\
Institution1\\
Institution1 address\\
{\tt\small firstauthor@i1.org}
\and
Second Author\\
Institution2\\
First line of institution2 address\\
{\tt\small secondauthor@i2.org}
}

\begin{document}
\input{sec/X_suppl}

\newpage
\clearpage
{
    \small
    \bibliographystyle{ieeenat_fullname}
    \bibliography{main}
}

\end{document}
